# Supplementary material for: Bilayer registry in a multicomponent asymmetric membrane : dependence on lipid composition and chain length
Source: arXiv:1309.4853 source file (2013-09-19)
Supplement: Supplementary file 1 [file SupplementaryInformation_JPCB9Sept2013.pdf]

# Supplementary Information

## Bilayer registry in a multicomponent asymmetric membrane : dependence on lipid composition and chain length

Anirban Polley, Satyajit Mayor and Madan Rao

### 1. Tabulation of force, torque and tension in model bilayers at equilibrium

From the MD simulation runs over the last 20 ns, we use the virial to calculate the net force $F_i = \int \partial_k \sigma_{ik}\, dv$ and torque $M_{ik} = \int (\partial_l \sigma_{il} x_k - \partial_l \sigma_{kl} x_i)\, dv$, where $i, j, k$ runs from $1, 2, 3$ (corresponding to the x, y and z components). This is to ensure that the model membrane is both force and torque balanced. In addition, to ensure that the membrane is tensionless, we compute the surface tension as $\gamma = \int \pi(z) dz$, where $\pi(z) = \frac{1}{2}\left(\overline{\sigma}_{xx}(z) + \overline{\sigma}_{yy}(z)\right) - \overline{\sigma}_{zz}(z)$, the lateral pressure, is integrated over the width of the bilayer [1, 2].

(a) We tabulate the values of the components of the force and torque for the asymmetric bilayer containing PSM in the lower leaflet, for different values of its relative concentration $x$, Table S1 and S2.

| x (in %) | $F_1(nN)$ | $F_2(nN)$ | $F_3(nN)$ |
|---|---|---|---|
| 33.3 | $0.663 \pm 0.14$ | $-0.839 \pm 0.09$ | $-0.196 \pm 0.02$ |
| 25.0 | $-0.334 \pm 0.06$ | $-0.476 \pm 0.07$ | $-0.282 \pm 0.03$ |
| 19.9 | $0.029 \pm 0.09$ | $-0.146 \pm 0.04$ | $-0.110 \pm 0.05$ |
| 14.3 | $-0.139 \pm 0.11$ | $0.083 \pm 0.12$ | $-0.200 \pm 0.15$ |
| 12.5 | $0.018 \pm 0.01$ | $0.141 \pm 0.04$ | $-0.301 \pm 0.05$ |
| 10.0 | $-0.123 \pm 0.02$ | $0.144 \pm 0.01$ | $-0.111 \pm 0.01$ |
| 9.1 | $-0.256 \pm 0.01$ | $0.180 \pm 0.09$ | $-0.299 \pm 0.08$ |
| 7.1 | $-0.055 \pm 0.03$ | $0.116 \pm 0.04$ | $-0.109 \pm 0.01$ |
| 5.9 | $-0.365 \pm 0.01$ | $-0.216 \pm 0.02$ | $-0.197 \pm 0.05$ |
| 4.5 | $0.298 \pm 0.11$ | $-0.371 \pm 0.09$ | $-0.136 \pm 0.01$ |

Table S1: Computed values of the components of the net force at different values of $x$, the relative concentration of PSM in the lower leaflet.

| x (in %) | $M_{12}(nN \cdot nm)$ | $M_{13}(nN \cdot nm)$ | $M_{23}(nN \cdot nm)$ |
|---|---|---|---|
| 33.3 | $6.136 \pm 0.128$ | $1.102 \pm 0.14$ | $-8.153 \pm 0.17$ |
| 25.0 | $-4.396 \pm 0.019$ | $-2.927 \pm 0.09$ | $-0.001 \pm 0.12$ |
| 19.9 | $-2.220 \pm 0.182$ | $-0.687 \pm 0.099$ | $-4.246 \pm 0.194$ |
| 14.3 | $-0.224 \pm 0.112$ | $1.184 \pm 0.106$ | $5.449 \pm 0.074$ |
| 12.3 | $-1.622 \pm 0.092$ | $5.411 \pm 0.091$ | $0.086 \pm 0.064$ |
| 10.0 | $-4.260 \pm 0.102$ | $1.403 \pm 0.076$ | $0.057 \pm 0.055$ |
| 9.1 | $-10.047 \pm 0.082$ | $-0.136 \pm 0.066$ | $4.677 \pm 0.081$ |
| 7.1 | $-5.499 \pm 0.099$ | $-1.226 \pm 0.064$ | $2.449 \pm 0.099$ |
| 5.9 | $-4.214 \pm 0.091$ | $-3.042 \pm 0.059$ | $1.702 \pm 0.048$ |
| 4.5 | $6.291 \pm 0.072$ | $4.094 \pm 0.086$ | $2.383 \pm 0.074$ |

Table S2: Computed values of the components of the net torque at different values of $x$, the relative concentration of PSM in the lower leaflet.

(b) We tabulate the values of the components of the force and torque for the asymmetric bilayer containing MSM in the lower leaflet, for different values of its relative concentration $x$, Table S3 and S4.

| x (in %) | $F_1(nN)$ | $F_2(nN)$ | $F_3(nN)$ |
|---|---|---|---|
| 14.3 | $-0.237 \pm 0.01$ | $0.084 \pm 0.08$ | $-0.118 \pm 0.05$ |
| 12.5 | $-0.105 \pm 0.02$ | $-0.586 \pm 0.01$ | $-0.202 \pm 0.01$ |
| 10.0 | $0.337 \pm 0.01$ | $0.133 \pm 0.05$ | $-0.139 \pm 0.03$ |
| 9.1 | $-0.154 \pm 0.02$ | $-0.103 \pm 0.01$ | $-0.171 \pm 0.01$ |
| 7.1 | $-0.140 \pm 0.01$ | $0.072 \pm 0.03$ | $-0.216 \pm 0.03$ |
| 5.9 | $-0.147 \pm 0.02$ | $0.075 \pm 0.01$ | $-0.098 \pm 0.04$ |
| 4.5 | $0.073 \pm 0.09$ | $-0.147 \pm 0.10$ | $-0.127 \pm 0.09$ |

Table S3: Computed values of the components of the net force at different values of $x$, the relative concentration of MSM in the lower leaflet.

| x (in %) | $M_{12}(nN \cdot nm)$ | $M_{13}(nN \cdot nm)$ | $M_{23}(nN \cdot nm)$ |
|---|---|---|---|
| 14.3 | $0.004 \pm 0.012$ | $-0.794 \pm 0.126$ | $0.551 \pm 0.029$ |
| 12.3 | $2.815 \pm 0.088$ | $1.332 \pm 0.141$ | $-0.795 \pm 0.088$ |
| 10.0 | $1.778 \pm 0.092$ | $2.729 \pm 0.179$ | $3.705 \pm 0.069$ |
| 9.1 | $-8.065 \pm 0.076$ | $-4.142 \pm 0.106$ | $-0.846 \pm 0.049$ |
| 7.1 | $-0.000 \pm 0.084$ | $4.058 \pm 0.079$ | $4.483 \pm 0.097$ |
| 5.9 | $-3.341 \pm 0.034$ | $2.889 \pm 0.059$ | $1.201 \pm 0.059$ |
| 4.5 | $-1.408 \pm 0.092$ | $-3.573 \pm 0.016$ | $-3.200 \pm 0.060$ |

Table S4: Computed values of the components of the net torque at different values of $x$, the relative concentration of MSM in the lower leaflet.

The tabulated values of force and torque components shown above are comparable to the values computed for the mechanically stable single component (POPC) symmetric bilayer [1]), where we found that $F_1 = 0.83 \pm 1.66$ nN, $F_2 = 0.27 \pm 1.14$ nN, $F_3 = -0.16 \pm 1.25$ nN and $M_{12} = 8.26 \pm 0.102$ nN $\cdot$ nm, $M_{13} = 10.74 \pm 0.066$ nN$\cdot$ nm, $M_{23} = 9.33 \pm 0.094$ nN$\cdot$ nm, at equilibrium. This suggests that the model membranes under study are both force and torque balanced.

(c) We tabulate the values of the surface tension for the asymmetric bilayer containing PSM / MSM in the lower leaflet, for different values of its relative concentration $x$, Table S5 and S6, respectively.

| x (in %) | $\gamma( bar \cdot nm)$ |
|---|---|
| 33.3 | $0.0324 \pm 0.009$ |
| 25.0 | $0.0466 \pm 0.0089$ |
| 19.9 | $-0.0342 \pm 0.0017$ |
| 14.3 | $0.0376 \pm 0.0017$ |
| 12.3 | $0.0169 \pm 0.0101$ |
| 10.0 | $0.0274 \pm 0.0017$ |
| 9.1 | $-0.0200 \pm 0.0157$ |
| 7.1 | $-0.0118 \pm 0.0112$ |
| 5.9 | $0.0204 \pm 0.0189$ |
| 4.5 | $0.0361 \pm 0.0151$ |

Table S5: Computed values of the surface tension $\gamma$ at different values of $x$, the relative concentration of PSM in the lower leaflet.

| x (in %) | $\gamma( bar \cdot nm)$ |
|---|---|
| 14.3 | $-0.0278 \pm 0.01$ |
| 12.5 | $0.0580 \pm 0.0211$ |
| 10.0 | $0.0132 \pm 0.0019$ |
| 9.1 | $-0.0395 \pm 0.0121$ |
| 7.1 | $-0.0504 \pm 0.0292$ |
| 5.9 | $0.0286 \pm 0.0089$ |
| 4.5 | $0.0478 \pm 0.0199$ |

Table S6: Computed values of the surface tension $\gamma$ at different values of $x$, the relative concentration of MSM in the lower leaflet.

The tabulated values of the surface tension shown above are comparable to the values computed for the tensionless single component (POPC) symmetric bilayer [1], where we found that $\gamma = 0.0204 \pm 0.0357$ bar$\cdot$ nm. This suggests that the model membranes under study are tensionless.

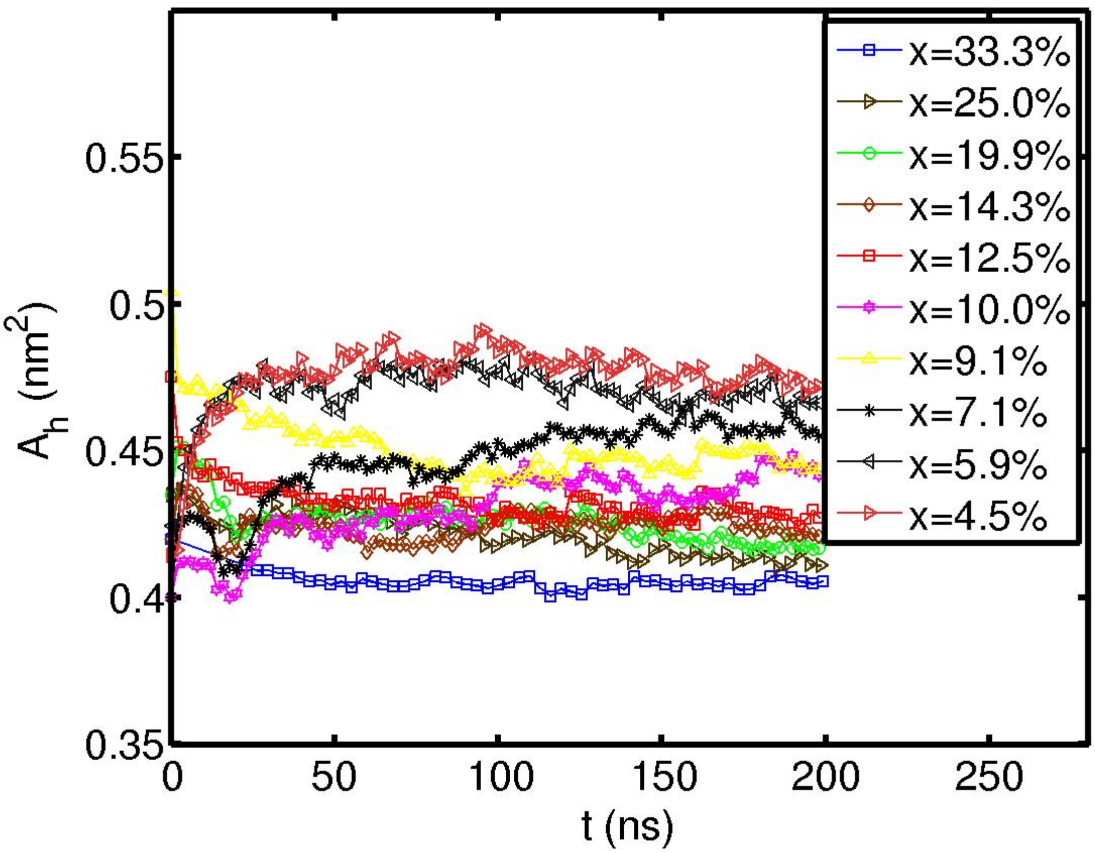


Figure S1: Mean area per lipid $A_h$ (mean calculated over all lipids in the bilayer membrane) versus time $t$ for simulations done at different $x$, the concentration of PSM in the lower leaflet. This shows that at times longer than $\approx 150\,$ns, the membrane is equilibrated.

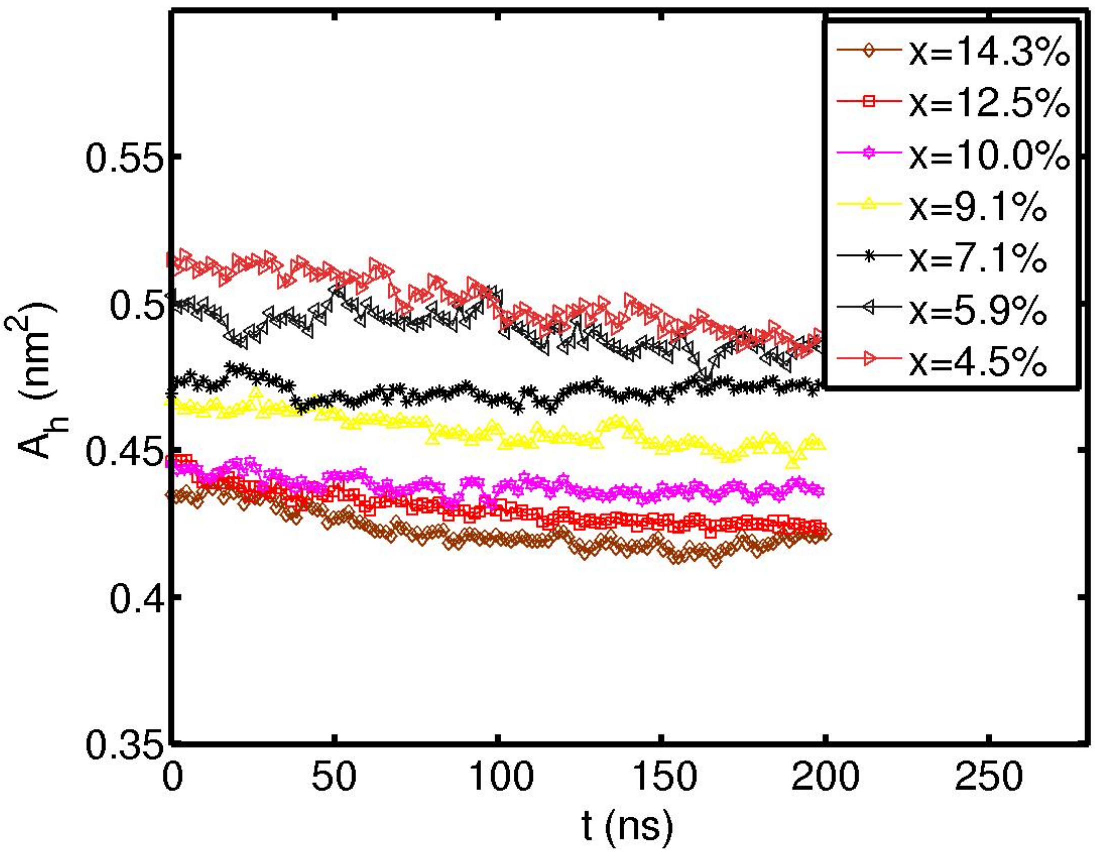


Figure S2: Mean area per lipid $A_h$ (mean calculated over all lipids in the bilayer membrane) versus time $t$ for simulations done at different $x$, the concentration of MSM in the lower leaflet. This shows that at times longer than $\approx 150$ ns, the membrane is equilibrated.

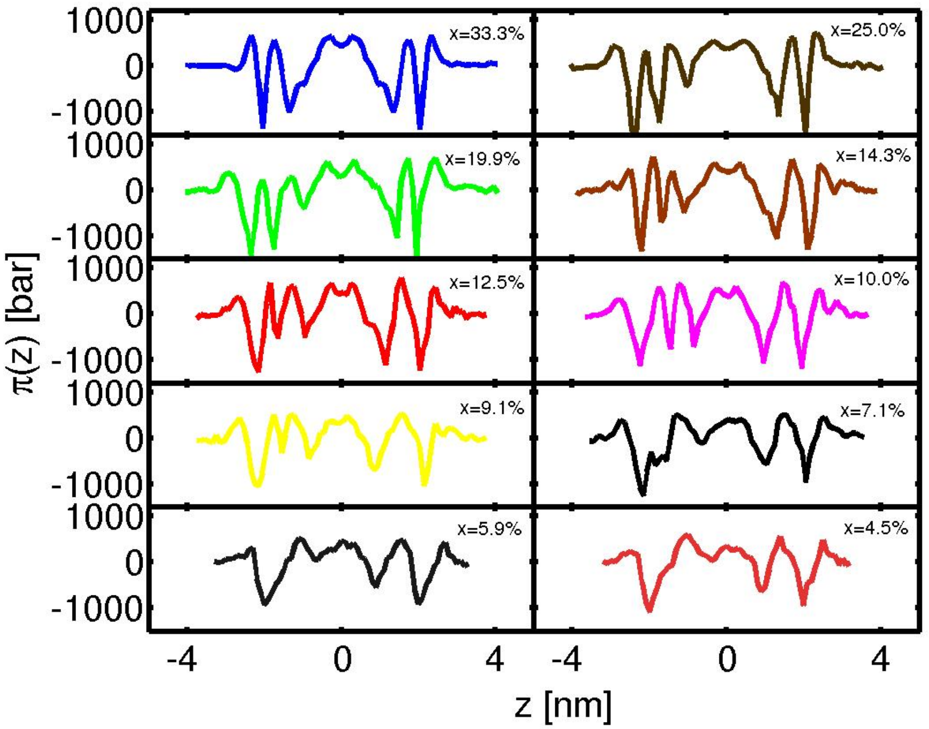


Figure S3: Mean lateral pressure, $\pi(z)$ versus $z$, the transverse coordinate of the membrane, at equilibrium for different values of $x$, the concentration of PSM in the lower leaflet.

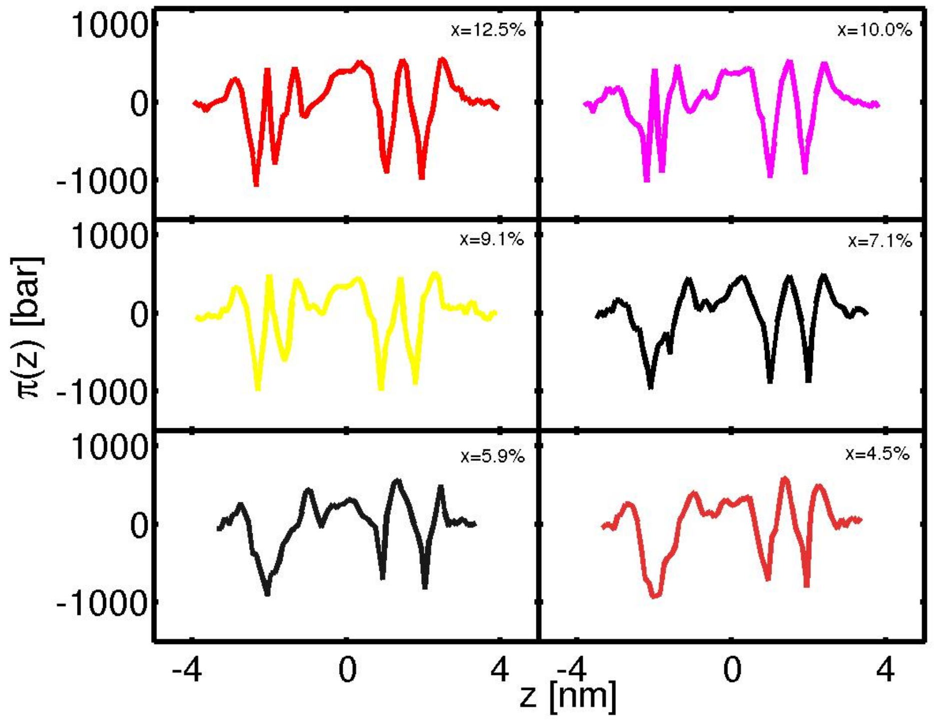


Figure S4: Mean lateral pressure, $\pi(z)$ versus $z$, the transverse coordinate of the membrane, at equilibrium for different values of $x$, the concentration of MSM in the lower leaflet.

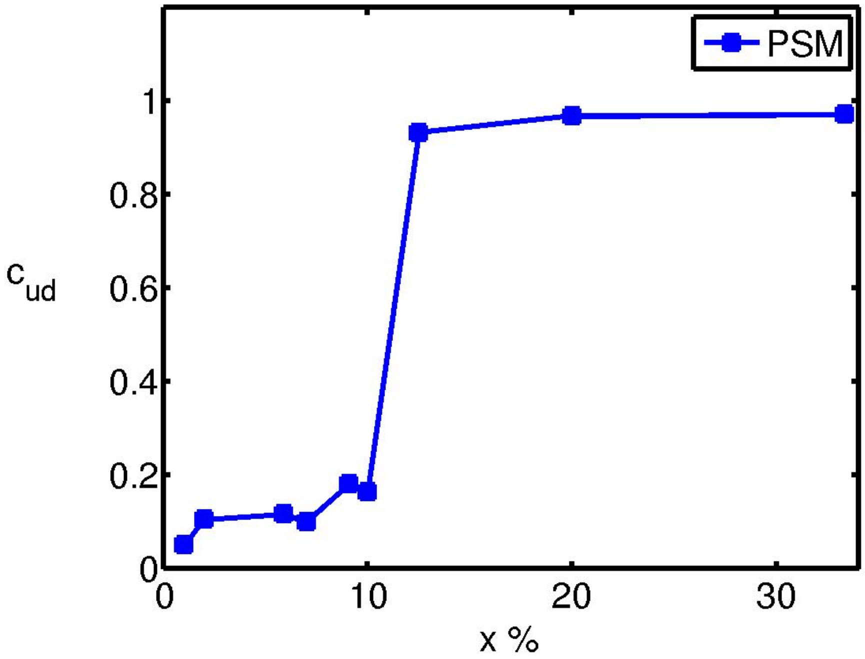


Figure S5: Transbilayer order parameter $C_{ud}$ for the symmetric bilayer, defined from the trans-bilayer correlation $C(\rho^u(r), \rho^d(r))$ (main manuscript) between the density of upper leaflet PSM and lower leaflet PSM (blue square) versus $x$, the concentration of PSM. The value of $C_{ud}$ is zero for small $x$ and jumps sharply at $x_c = 10\%$, coinciding with the first-order phase transition of the symmetric bilayer shown in Fig. 1 (main manuscript).

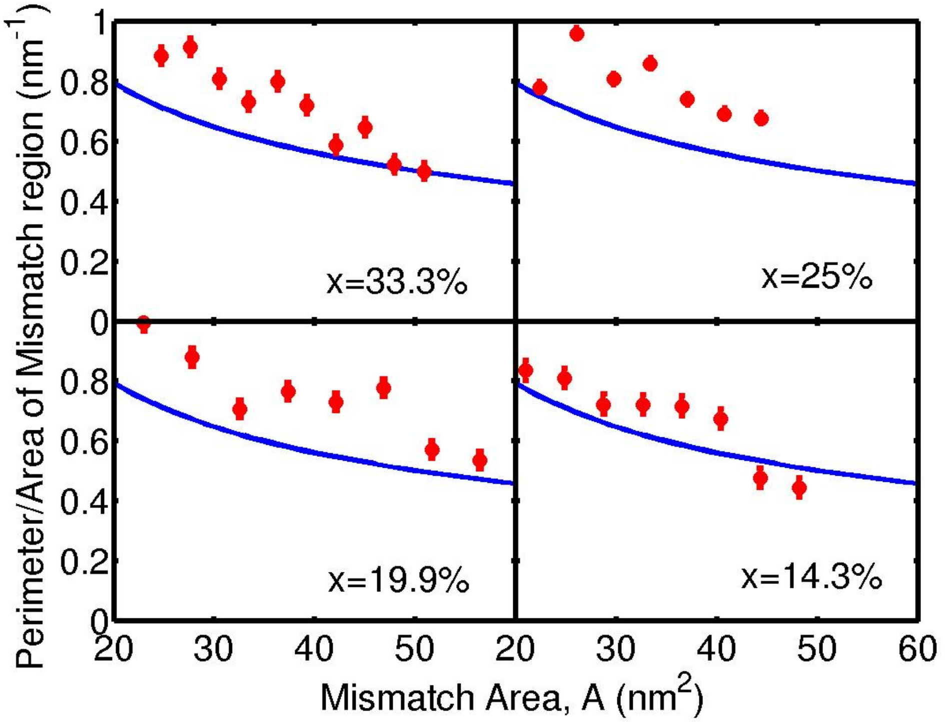


Figure S6: The ratio of the perimeter to area of the mismatch regions versus mismatch area $A$ (defined in main text) at equilibrium for different values of $x$, the concentration of PSM in the lower leaflet. The smooth line (blue) is a plot of the perimeter/area for a circular domain of area $A$ and goes as $2\sqrt{\pi/A}$. The fact that the simulation data (red dots) is above this line, indicates deviations from circularity.

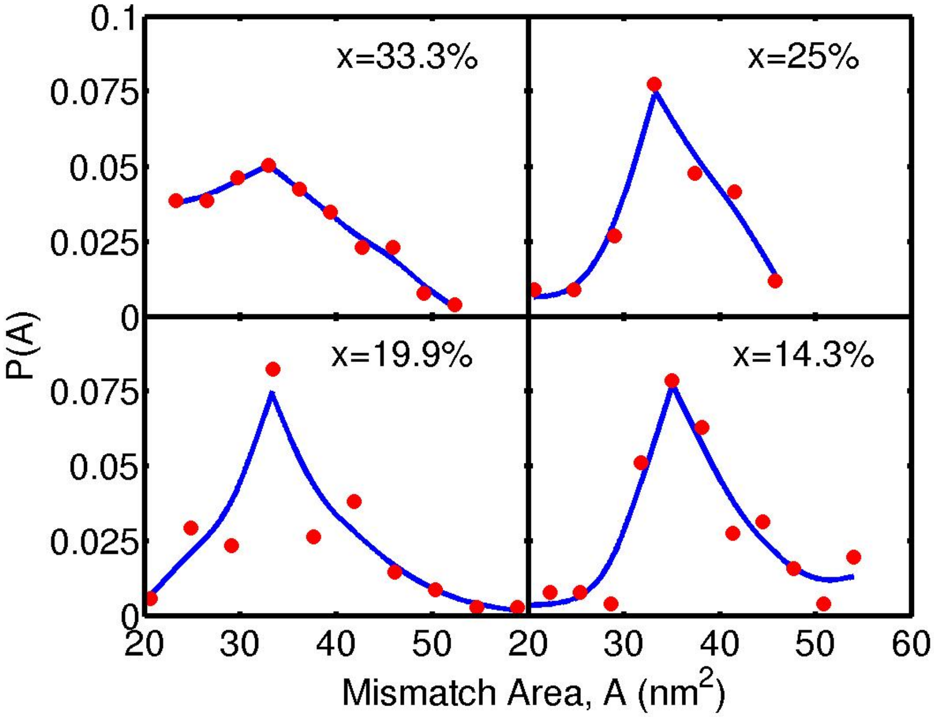


Figure S7: Probability $P(A)$ of the mismatch area $A$ at equilibrium for different values of $x$, the concentration of PSM in the lower leaflet. The smooth line (blue) is a cubic spline fit to the data (red dots).

# References


[1] A Polley, S Vemparala, and M Rao. *J Phys Chem B.* **2012**, 116, 13403–10.

[2] Niemela, P. S.; Ollila, S.; Hyvonen, M. T.; Karttunen, M. and Vattulainen, I. *Plos Comput Biol* **2007**, 3, 0304 – 0312.
